# Supplementary material for: Policy-Induced Self-Supervision Improves Representation Finetuning in Visual RL
Source: arXiv:2302.06009 source file (2023-02-12)
Supplement: Supplementary file 1 [file code_release.tex]

\section{Code Release}
\label{sec:code}

Together with our submission, we release example code to implement \pisco in the \texttt{code/} directory of the \supp.
We plan to publicly release complete implementations, together with examples for the pretrain-and-transfer pipeline.
We describe the main files below.

\begin{itemize}
    \item \texttt{msr\_jump.py}: our GPU implementation of \jump tasks.
    \item \texttt{ppo\_pisco.py}: our PyTorch~\citep{Paszke2019-fx} implementation of \pisco on top of PPO.
    \item \texttt{drqv2\_pisco.py}: our PyTorch~\citep{Paszke2019-fx} implementation of \pisco on top of DrQ-v2.
\end{itemize}
